# Supplementary material for: A Distributed Adaptive Algorithm for Non-Smooth Spatial Filtering Problems in Wireless Sensor Networks
Source: arXiv:2403.08658 source file (2024-03-13)
Supplement: Supplementary file 1 [file supplementary.tex]

\newcommand{\seq}[2]{(#1^i)_{i\in #2}}
\newcommand{\N}{\mathbb{N}}

\subsection{Structure of $C_q(\X)$}

When computing $C_q^T(X)U$, where $U$ is any block matrix (or vector), whose blocks of rows have the same number of rows as the blocks $X_k$ of $X$, we expect the following, according to the update rules \eqref{eq:update_rule_q}-\eqref{eq:update_rule_k}:
\begin{itemize}
    \item The first block of $M_q$ rows of $C_q(X)$ should select the $q$-th block of $U$.
    \item The remaining blocks should produce $\X_k^T U_k$.
\end{itemize}
Defining 
\begin{equation}
    \begin{split}
        \Gamma_q &= 
        \begin{bmatrix}
            0 & \dots & I_{M_q} & \dots & 0
        \end{bmatrix}^T,\\
        \Theta_{-q}(X) &= 
        \begin{bmatrix}
            X_1 & 0 & \dots  & \dots & 0\\
             & \ddots & \dots & \dots & \vdots \\
            0 & \dots & X_{q-1} & \dots & 0 
        \end{bmatrix} \textrm { and, }\\
        \Theta_{+q}(X) &=
        \begin{bmatrix}
            0 & \dots & X_{q+1} & \dots & 0 \\
            \vdots & \ddots & \dots & \ddots &  \\
            0 & \dots & 0 & \dots & X_K 
        \end{bmatrix}
    \end{split}
\end{equation}
We can express $C_q(X)$ as
\begin{equation}
    \label{eq:def_Cq}
    C_q(X)=\left[\Gamma_q \;|\; \Theta_{-q}(X)\;|\; \Theta_{+q}(X) \right].
\end{equation}
Indeed, $\Gamma_q$ selects the $M_q$ rows associated with node $q$ and prepends them to the output, while the matrices $\Theta_{-q}(X)$ and $\Theta_{+q}(X)$ select the blocks associated with the nodes before and after node $q$, respectively, and mutliplyinng them by the corresponding $\X_k$'s. Note tgat $C_q$ is a linear, and hence continuous, map.

\subsection{Continuity of Quadratic Orthogonality Constraints}
$\E{\y\y^T}$ being positive definite, it can be uniquely factored as $\E{\y\y^T}
\triangleq RR^T$ \cite{Horn2012},
then \eqref{eq:quad_constraints} can be expressed as,
\begin{equation}
        \label{eq:quad_constraints_2}
        \begin{split}
                \mc{X}(\bm{y}) &= \{ \X \;|\; Y^TY ={I},
                Y=R^T{X} \}\\
                               & = \{
                                       \X=R^{-T} Y \;|\;
                                       Y^TY ={I} \},
\end{split}
\end{equation}
As the Cholesky decomposition and matrix inverse are continuous on the set of positive definite
matrices \cite{schatzman2002numerical, rakovcevic1997continuity}, $\mc{X}(\cdot)$ is a continuous map (by
composition). 

\subsection{Proof of Lemma \ref{lem:Rq_cont}}
\label{apx:proof_Rq_cont}
\begin{proof}
        The map $\mc{R}_q$ is merely the composition of several continuous maps. We denote $C^D_q(\X,\cdot)$ the linear map which given the set 
        \begin{equation}
                \mc{D}\triangleq \{D_{j,k}\;|\; j\in\mc{J}_{E}^k\cup \mc{J}_{I}^k,\;k\in\mc{K}\}
        \end{equation}
        produces
        \begin{multline}
                \widetilde{\mc{D}}\triangleq \{X^T_k D_{j,k}\;|\;j\in \mc{J}_{E}^k\cup \mc{J}_{I}^k,\;k\in\mc{K}\setminus\{q\}\}\\\cup \{D_{j,q}\;|\;j\in \mc{J}_{E}^q\cup \mc{J}_{I}^q\}.
        \end{multline}

        Indeed, $U\in\mc{R}_q(\X)$ implies that $\exists \lX: U = C_q(\X)\lX$ and $U\in\mathcal{X}(\y,\C)$, and hence $$C_q(\X)\lX\in\mathcal{X}(\y,\C)$$
        By associativity and the definition \eqref{eq:constraints_map} of $\mc{X}(\cdot,\cdot)$\footnote{This is with a slight abuse of notation. The maps $\mc{X}(\y,\mc{D})$ and $\mc{X}(C_q(\X)^T\y, C_q(\X)^T\C)$ are technically different maps as their input spaces have different dimensions.}, 
        \begin{equation}
                \begin{split}
                        C_q(\X)\lX\in\mathcal{X}(\y,\mc{D})&\Leftrightarrow \lX \in \mc{X}(C_q(\X)^T\y,C^D_q(\X,\mc{D}))\\
                                                       &\Leftrightarrow U\in C_q(\X)\mc{X}(C_q(\X)^T\y, C^D_q(\X,\mc{D}))\\
                                                       &\Leftrightarrow U\in \mc{R}_q(\X)
                \end{split}
        \end{equation}
        where the left-multiplication of a set by a matrix must be understood as an element-wise operation. Therefore 
        \begin{equation}
                \mc{R}_q(\X) = C_q(\X)\mc{X}(C_q(\X)^T\y, C^D_q(\X,\mc{D})),
        \end{equation}
        which is continuous by the composition of $\mc{X}$, $C_q$ ($C_q$ being trivially continuous as its blocks are simply sub-blocks of its argument, see \eqref{eq:def_Cq}) and $\X\mapsto C^D_q(\X,\mc{D})$ \cite[Theorem 17.23]{Charalambos2013}.
\end{proof}

\subsection{Useful Lemmas}
\label{apx:useful_lemmas}
\begin{lemma}
        \label{lem:conv_to_acc}
        Let $\seq{\X}{\N}$ be some sequence in a metric space. Then 
        \begin{equation}
                \label{eq:conv_to_acc}
        \lim_{i\to\infty}\min_{\accX\in\textrm{Acc }\seq{\X}{\N}} \norm{X^i-\accX}_F=0,
\end{equation}
        i.e. $\seq{\X}{\N}$ converges to the set of its accumulation points.
\end{lemma}
\begin{proof}
        This statement is in fact the definition of an accumulation point in hiding. A point
        $$\accX\in\textrm{Acc }\seq{\X}{\N}$$
        is an accumulation point if and only if \cite{rudin1976principles} there exists some index set $\mc{I}$ such that 
        \begin{equation}
                \label{eq:def_accu}
        \lim_{i\in\mc{I}\to\infty} \norm{\X^i - \accX}_F = 0.
\end{equation}
        Assume that \eqref{eq:conv_to_acc} is not true. Then there exists some $\varepsilon >0$ such that 
        \begin{equation}
        \lim_{i\to\infty}\min_{\accX\in\textrm{Acc }\seq{\X}{\N}} \norm{X^i-\accX}_F\geq \varepsilon.
        \end{equation}
        In particular,  for any $\accX\in\textrm{Acc }\seq{\X}{\N}$,
        \begin{equation}
        \lim_{i\to\infty} \norm{X^i-\accX}_F\geq \varepsilon,
        \end{equation}
        which is in contradiction with \eqref{eq:def_accu}.
\end{proof}

\begin{lemma}
    \label{lem:exists_Q}
    Let $\seq{q}{\N}$ be a sequence such that $q^i\in\mc{K}$, a finite set. Then for any $i$ there is some $Q<\infty$ such that $\textrm{Acc } \seq{q}{\N}\subseteq \{q^i,\dots,q^{i+Q}\} $.
\end{lemma}
\begin{proof}
 By definition, for any $q\in\textrm{Acc } \seq{q}{\N}$, there is some $Q_q<\infty$ such that for any $i$, $q\in\{q^i,\dots,q^{i+Q_q}\}$. If this were not the case, $q$ could not be an accumulation point as there would always be a finite non-zero distance between $q^j$ and $q$ for $j\geq i$. As a result, choosing $Q=\max_q Q_q$ ensures that $q\in\{q^i,\dots,q^{i+Q}\}$ for any $q\in\textrm{Acc } \seq{q}{\N}$ and hence  $\textrm{Acc } \seq{q}{\N}\subseteq \{q^i,\dots,q^{i+Q}\} $.
\end{proof}
